# Supplementary material for: Visual Dialog
Source: arXiv:1611.08669 source file (2017-08-01)
Supplement: Supplementary file 1 [file supp.tex]

%%%%%%%%%%%%%%%%%%%%%%%%%%%%%%%%%%%%%%%%%%%%%%%%%%%%%%%%%%%
\section{Qualitative Examples from \vd}
\label{sec:qual}
%%%%%%%%%%%%%%%%%%%%%%%%%%%%%%%%%%%%%%%%%%%%%%%%%%%%%%%%%%%
% Make this a 2x2 figure
\begin{figure*}[ht]
\centering
\begin{subfigure}[t]{0.48\textwidth}
	\centering
	\includegraphics[trim={0cm 0cm 0cm 0cm},clip, width=\columnwidth]{figures/Example1.png}
\end{subfigure}
\begin{subfigure}[t]{0.48\textwidth}
	\centering
	\includegraphics[trim={0cm 0cm 0cm 0cm},clip, width=\columnwidth]{figures/Example2.png}
\end{subfigure}

\begin{subfigure}[t]{0.48\textwidth}
	\centering
	\includegraphics[trim={0cm 0cm 0cm 0cm},clip, width=\columnwidth]{figures/Example3.png}
\end{subfigure}
\begin{subfigure}[t]{0.48\textwidth}
	\centering
	\includegraphics[trim={0cm 0cm 0cm 0cm},clip, width=\columnwidth]{figures/Example4.png}
\end{subfigure}
%\vspace{-2pt}
\label{fig:vd-examples-4}
\caption{Examples from \vd}
\end{figure*}

%\begin{figure}[thbp]
%\centering
%\includegraphics[width=1\linewidth]{figures/Example1.png}
%\end{figure}
%
%\begin{figure}[thbp]
%\centering
%\includegraphics[width=1\linewidth]{figures/Example2.png}
%\end{figure}
%
%\begin{figure}[thbp]
%\centering
%\includegraphics[width=1\linewidth]{figures/Example3.png}
%\end{figure}
%
%\begin{figure}[thbp]
%\centering
%\includegraphics[width=1\linewidth]{figures/Example4.png}
%\end{figure}

%%%%%%%%%%%%%%%%%%%%%%%%%%%%%%%%%%%%%%%%%%%%%%%%%%%%%%%%%%%
\section{Additional Analysis of \vd}
\label{sec:analysis}
%%%%%%%%%%%%%%%%%%%%%%%%%%%%%%%%%%%%%%%%%%%%%%%%%%%%%%%%%%%

\begin{figure}[h]
\includegraphics[width=\linewidth]{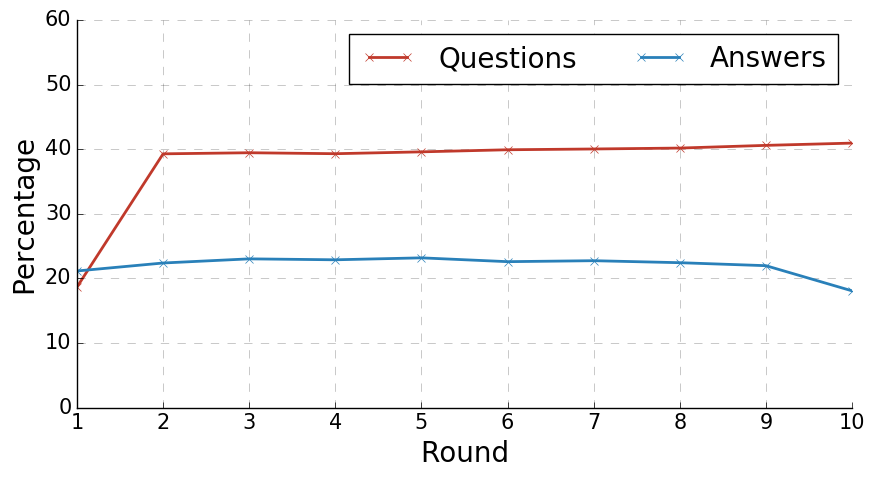}
\caption{Percentage of QAs with pronouns for different rounds}
\label{fig:quesPronouns}
\end{figure}

\begin{figure}[thbp]%{r}{0.5\linewidth}
\centering
\includegraphics[width=\linewidth]{figures/binaryQA.png}
\caption{Binary Q/A per round. \todo{Lots of space, but not sure if anything significant is being conveyed. Summarize 
a single number in text and move this to supplement. No figure already made should go to waste. It should just go to supplement.}}
\label{fig:binaryQA}
\end{figure}

\begin{figure}
    \centering
    \includegraphics[width=\linewidth]{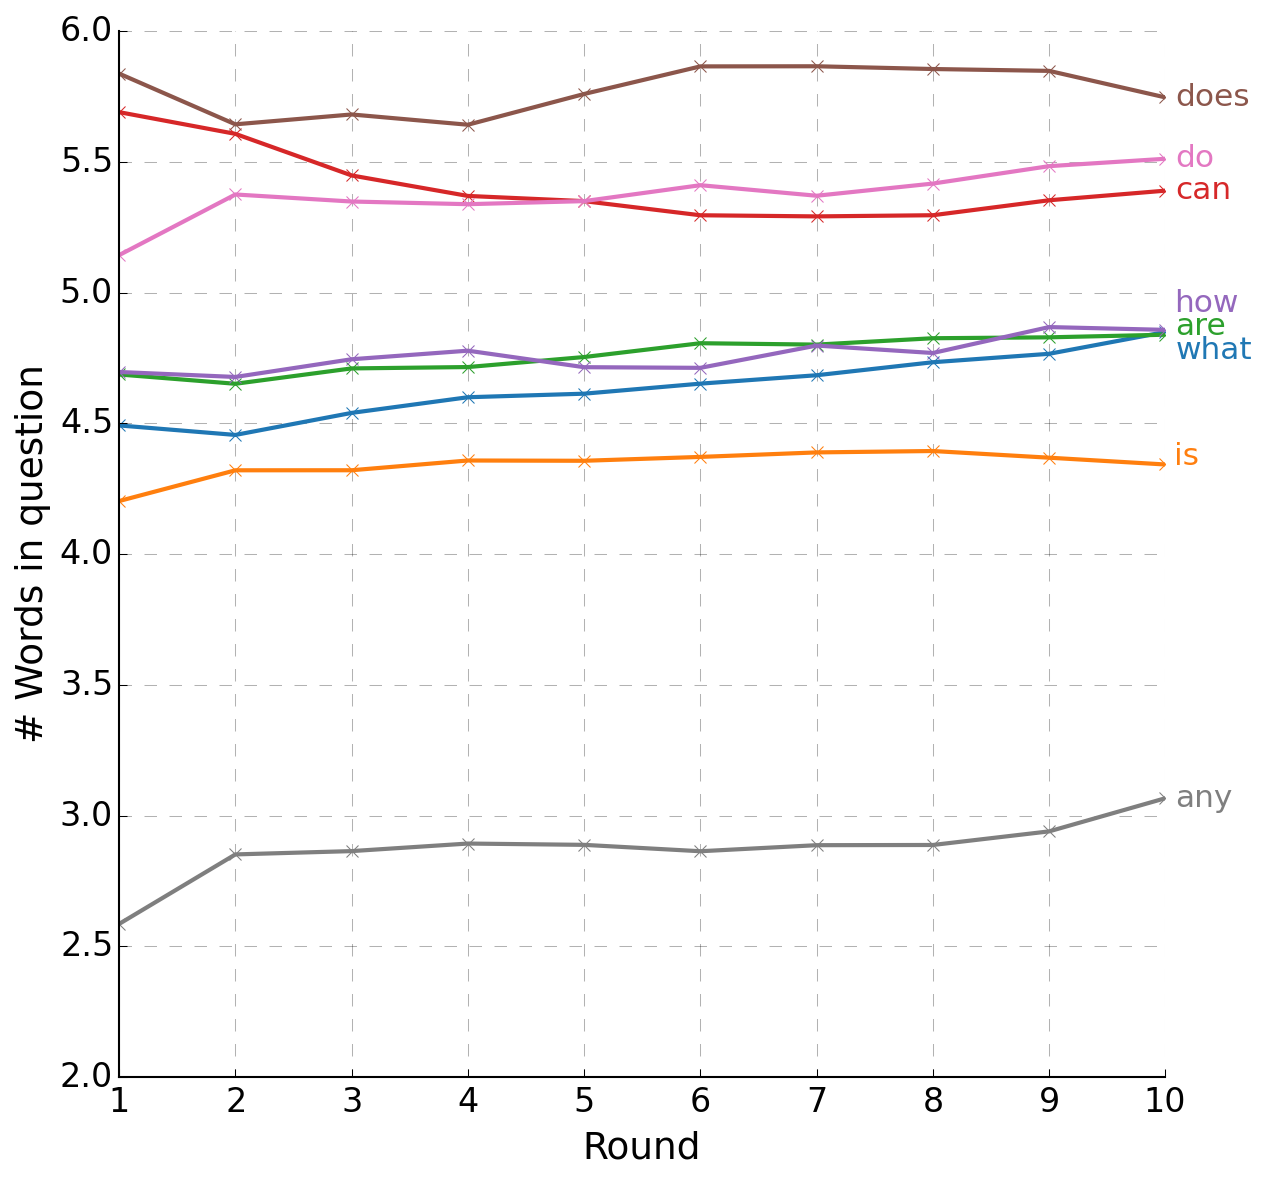}
    \caption{Question lengths by type and round. Average length of question by type is fairly consistent across rounds. Questions starting with `any' (`any people?', `any other fruits?', etc.) tend to be the shortest.}
    \label{fig:qlength_type_round}
\end{figure}

\begin{figure}
    \centering
    \includegraphics[width=\linewidth]{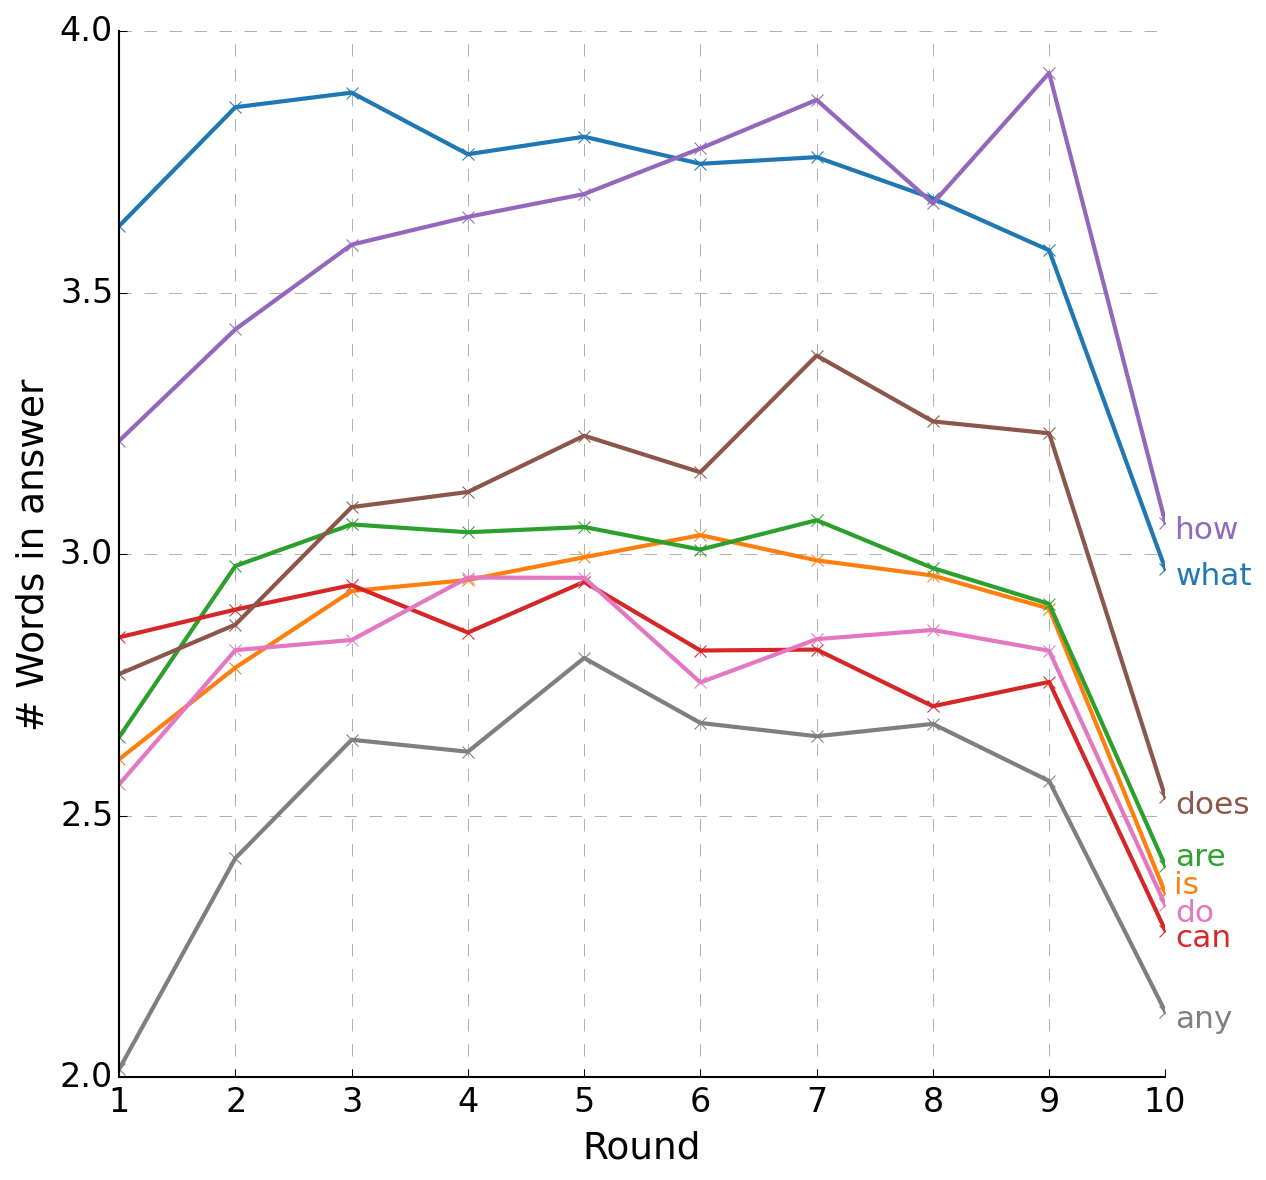}
    \caption{Answer lengths by question type and round. Across question types, average response length tends to be longest in the middle of the conversation.}
    \label{fig:alength_type_round}
\end{figure}

\begin{figure}
    \centering
    \includegraphics[width=\linewidth]{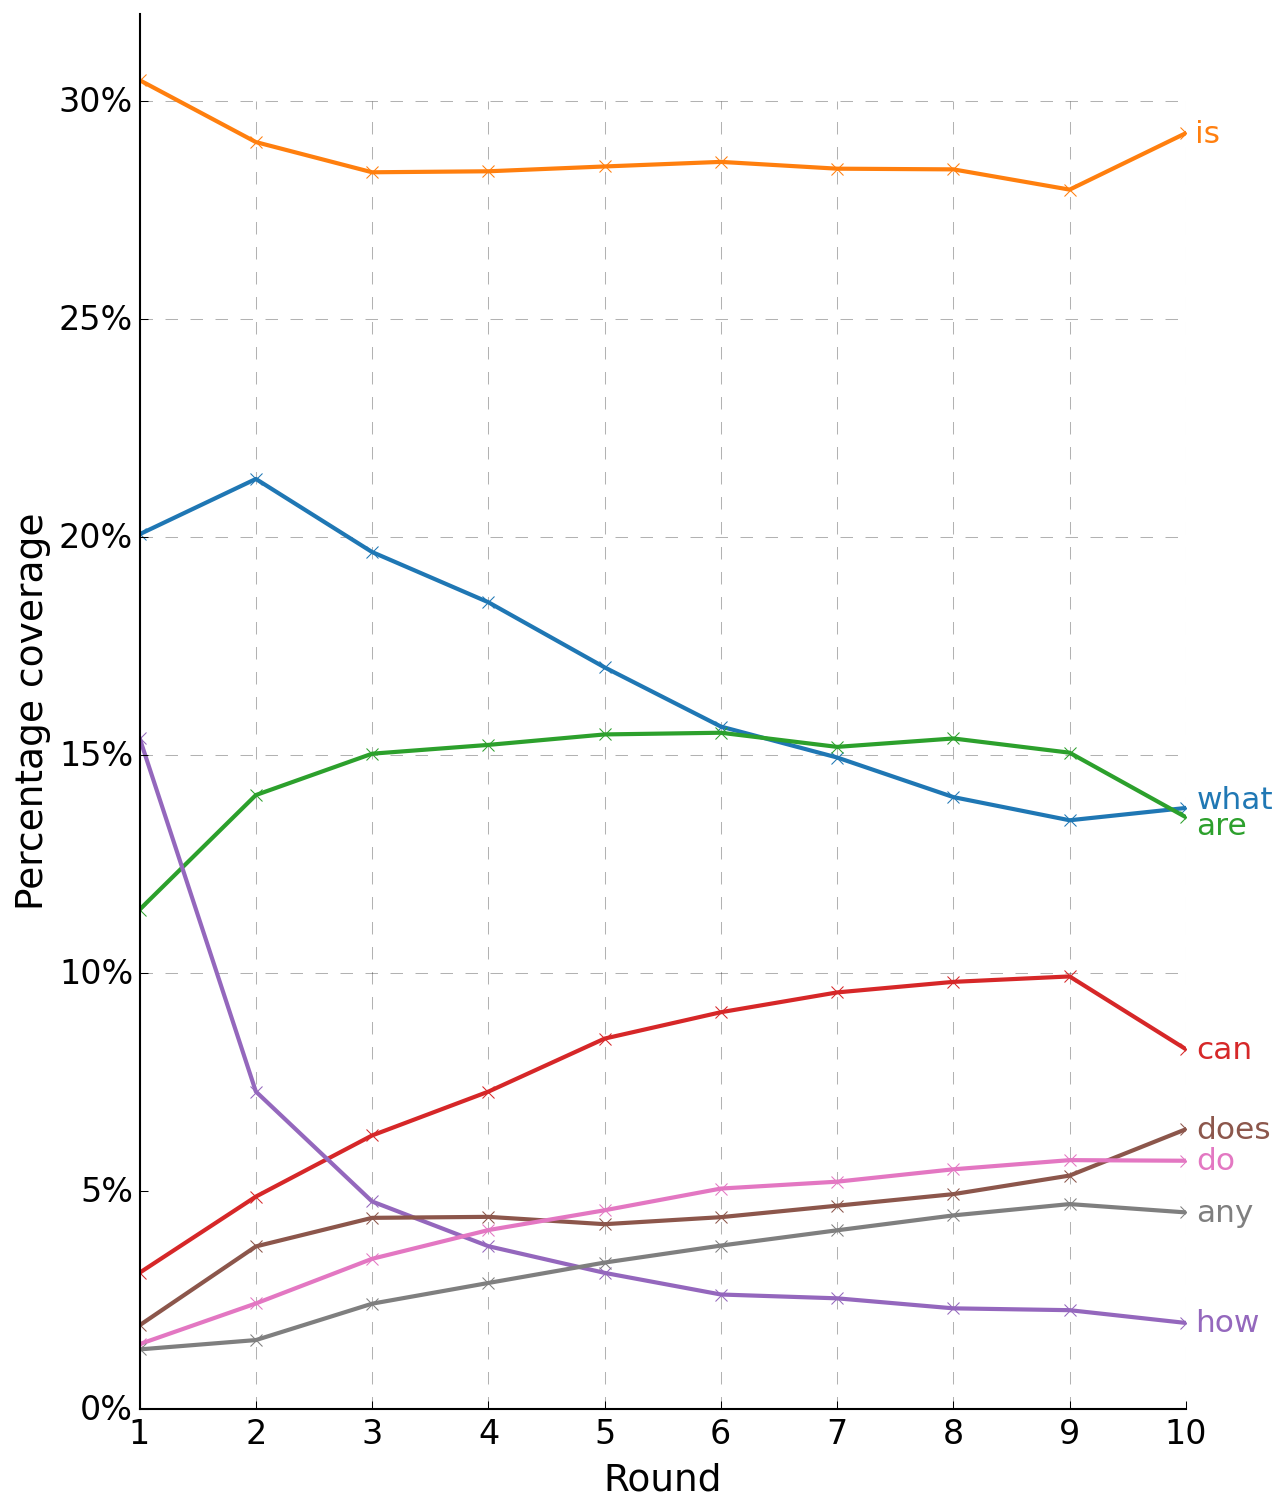}
    \caption{Percentage of question types per round}
    \label{fig:qtype_round}
\end{figure}

\begin{table*}[t]
\small
\centering
%\begin{scriptsize}
\begin{tabular}{lrrccccccccc}
\hline
& \textbf{\# QA} & \textbf{\# Images} & \textbf{AvgQLen} & \textbf{AvgALen} & \textbf{LongAns} & \textbf{TopAns} & \textbf{HumanPerf} & \textbf{COCO} & \textbf{MC} \\
\hline
DAQUAR~\cite{malinowski_nips14} & 12,468 & 1,447 & 11.5$\,\pm\,$2.4 & 1.2$\,\pm\,$0.5 & 3.4\% & 96.4\% &  &  &\\
Visual Madlibs~\cite{yu_iccv15} & 56,468 & 9,688 & 4.9$\,\pm\,$2.4 & 2.8$\,\pm\,$2.0 & 47.4\% & 57.9\% &  &  & \\
COCO-QA~\cite{ren_nips15} & 117,684 & 69,172 & 8.7$\,\pm\,$2.7 & 1.0$\,\pm\,$0 & 0.0\% & 100\% &  &\\
Baidu~\cite{gao_nips15} & 316,193 & 316,193 & - & - & - & - & & $\checkmark$ & \\
VQA~\cite{antol_iccv15} & 614,163 & 204,721 & 6.2$\,\pm\,$2.0 & 1.1$\,\pm\,$0.4 & 3.8\% & 82.7\% & $\checkmark$ & $\checkmark$ & $\checkmark$\\
Visual7W~\cite{zhu_cvpr16} & 327,939 & 47,300 & 6.9$\,\pm\,$2.4 & 2.0$\,\pm\,$1.4 & 27.6\% & 63.5\% & $\checkmark$ & $\checkmark$ & $\checkmark$\\
\hline
\vd (Ours) & 680,000 & 68,000 & 4.64$\,\pm\,$0 & 3.08$\,\pm\,$0 & NA & 58.1\% & $\checkmark$ & $\checkmark$ & $\checkmark$\\
\hline
\end{tabular}
\label{table:comparisons_between_datasets}
\caption{Comparison of existing datasets with \vd}
%\end{scriptsize}
\end{table*}

\todo{write descriptions of these figures. Pull out trends. Repeat them in captions.}

%%%%%%%%%%%%%%%%%%%%%%%%%%%%%%%%%%%%%%%%%%%%%%%%%%%%%%%%%%%
%\vspace{\sectionReduceBot}
\section{Supplementary}
\label{sec:supplementary}
%\vspace{\sectionReduceBot}
%%%%%%%%%%%%%%%%%%%%%%%%%%%%%%%%%%%%%%%%%%%%%%%%%%%%%%%%%%%
\sk{
    \todo{How frequently are new entities discovered that are not a part of the caption ?}
}

%%%%%%%%%%%%%%%%%%%%%%%%%%%%%%%%%%%%%%%%%%%%%%%%%%%%%%%%%%%
\begin{figure*}[h]
\centering
\begin{subfigure}[b]{0.32\textwidth}
	\centering
	\includegraphics[height=0.5\textwidth]{figures/amt_interaction.pdf}
	\caption{Live chat interface on AMT.}
	\label{fig:pascalExamples}
\end{subfigure}
\quad
\begin{subfigure}[b]{0.32\textwidth}
	\centering
	\includegraphics[height=0.5\textwidth]{figures/final/amt_questioner.png}
	\caption{What the `questioner' sees.}
	\label{fig:pascalExamples}
\end{subfigure}
\begin{subfigure}[b]{0.32\textwidth}
	\centering
	\includegraphics[height=0.5\textwidth]{figures/final/amt_answerer.png}
	\caption{What the `answerer' sees.}
	\label{fig:pascalExamples}
\end{subfigure}
%\vspace{-2pt}
%\vspace{\captionReduceTop}
\caption{Collecting visually-grounded dialog data on Amazon Mechanical Turk via a live chat interface
where one person is assigned the role of `questioner' and the second person is the `answerer'.}
%  \vspace{-5pt}
\label{fig:vd_amt}
\vspace{\captionReduceBot}
\end{figure*}

%%%%%%%%%%%%%%%%%%%%%%%%%%%%%%%%%%%%%%%%%%%%%%%%%%%%%%%%%%%
%\vspace{\sectionReduceBot}
\section{Human Studies}
\label{sec:human_supp}
%\vspace{\sectionReduceBot}
%%%%%%%%%%%%%%%%%%%%%%%%%%%%%%%%%%%%%%%%%%%%%%%%%%%%%%%%%%%

\ad{
    We conduct studies on AMT to quantitatively evaluate human performance on this task.
    While machines are evaluated on retrieval from 100 candidate answers, ranking 100 options for a given question is tedious for humans.
    Instead, we ask humans to rank 10 options consisting of top-9 predictions from our best-performing discriminative model (LF-QIH-Dis from \reftab{table:model_results}) and the ground-truth.
    This setup sufficiently captures the difference in machine and human performance while being cognitively lighter.
    We perform this task for all combinations of \{with image, without image\}$\times$\{with history, without history\} uniformly across rounds on 1000 visual dialogs from the \val set.
    Results from our studies are summarized in \reftab{table:model_results}.
    \reffig{fig:human_acc} \todo{update figure, possibly move figure to supp if less space} shows fine-grained human accuracy trends across rounds.
    We see that without image, humans perform better when they have access to dialog history.
    As expected, this gap narrows down when they have access to the image.
    However in both cases, dialog history improves performance, which serves as evidence that aspects unique to \vd (coreferences, consistency and speaker personality) provide useful signals.
}

\begin{figure}[]
    \centering
    \includegraphics[width=\linewidth]{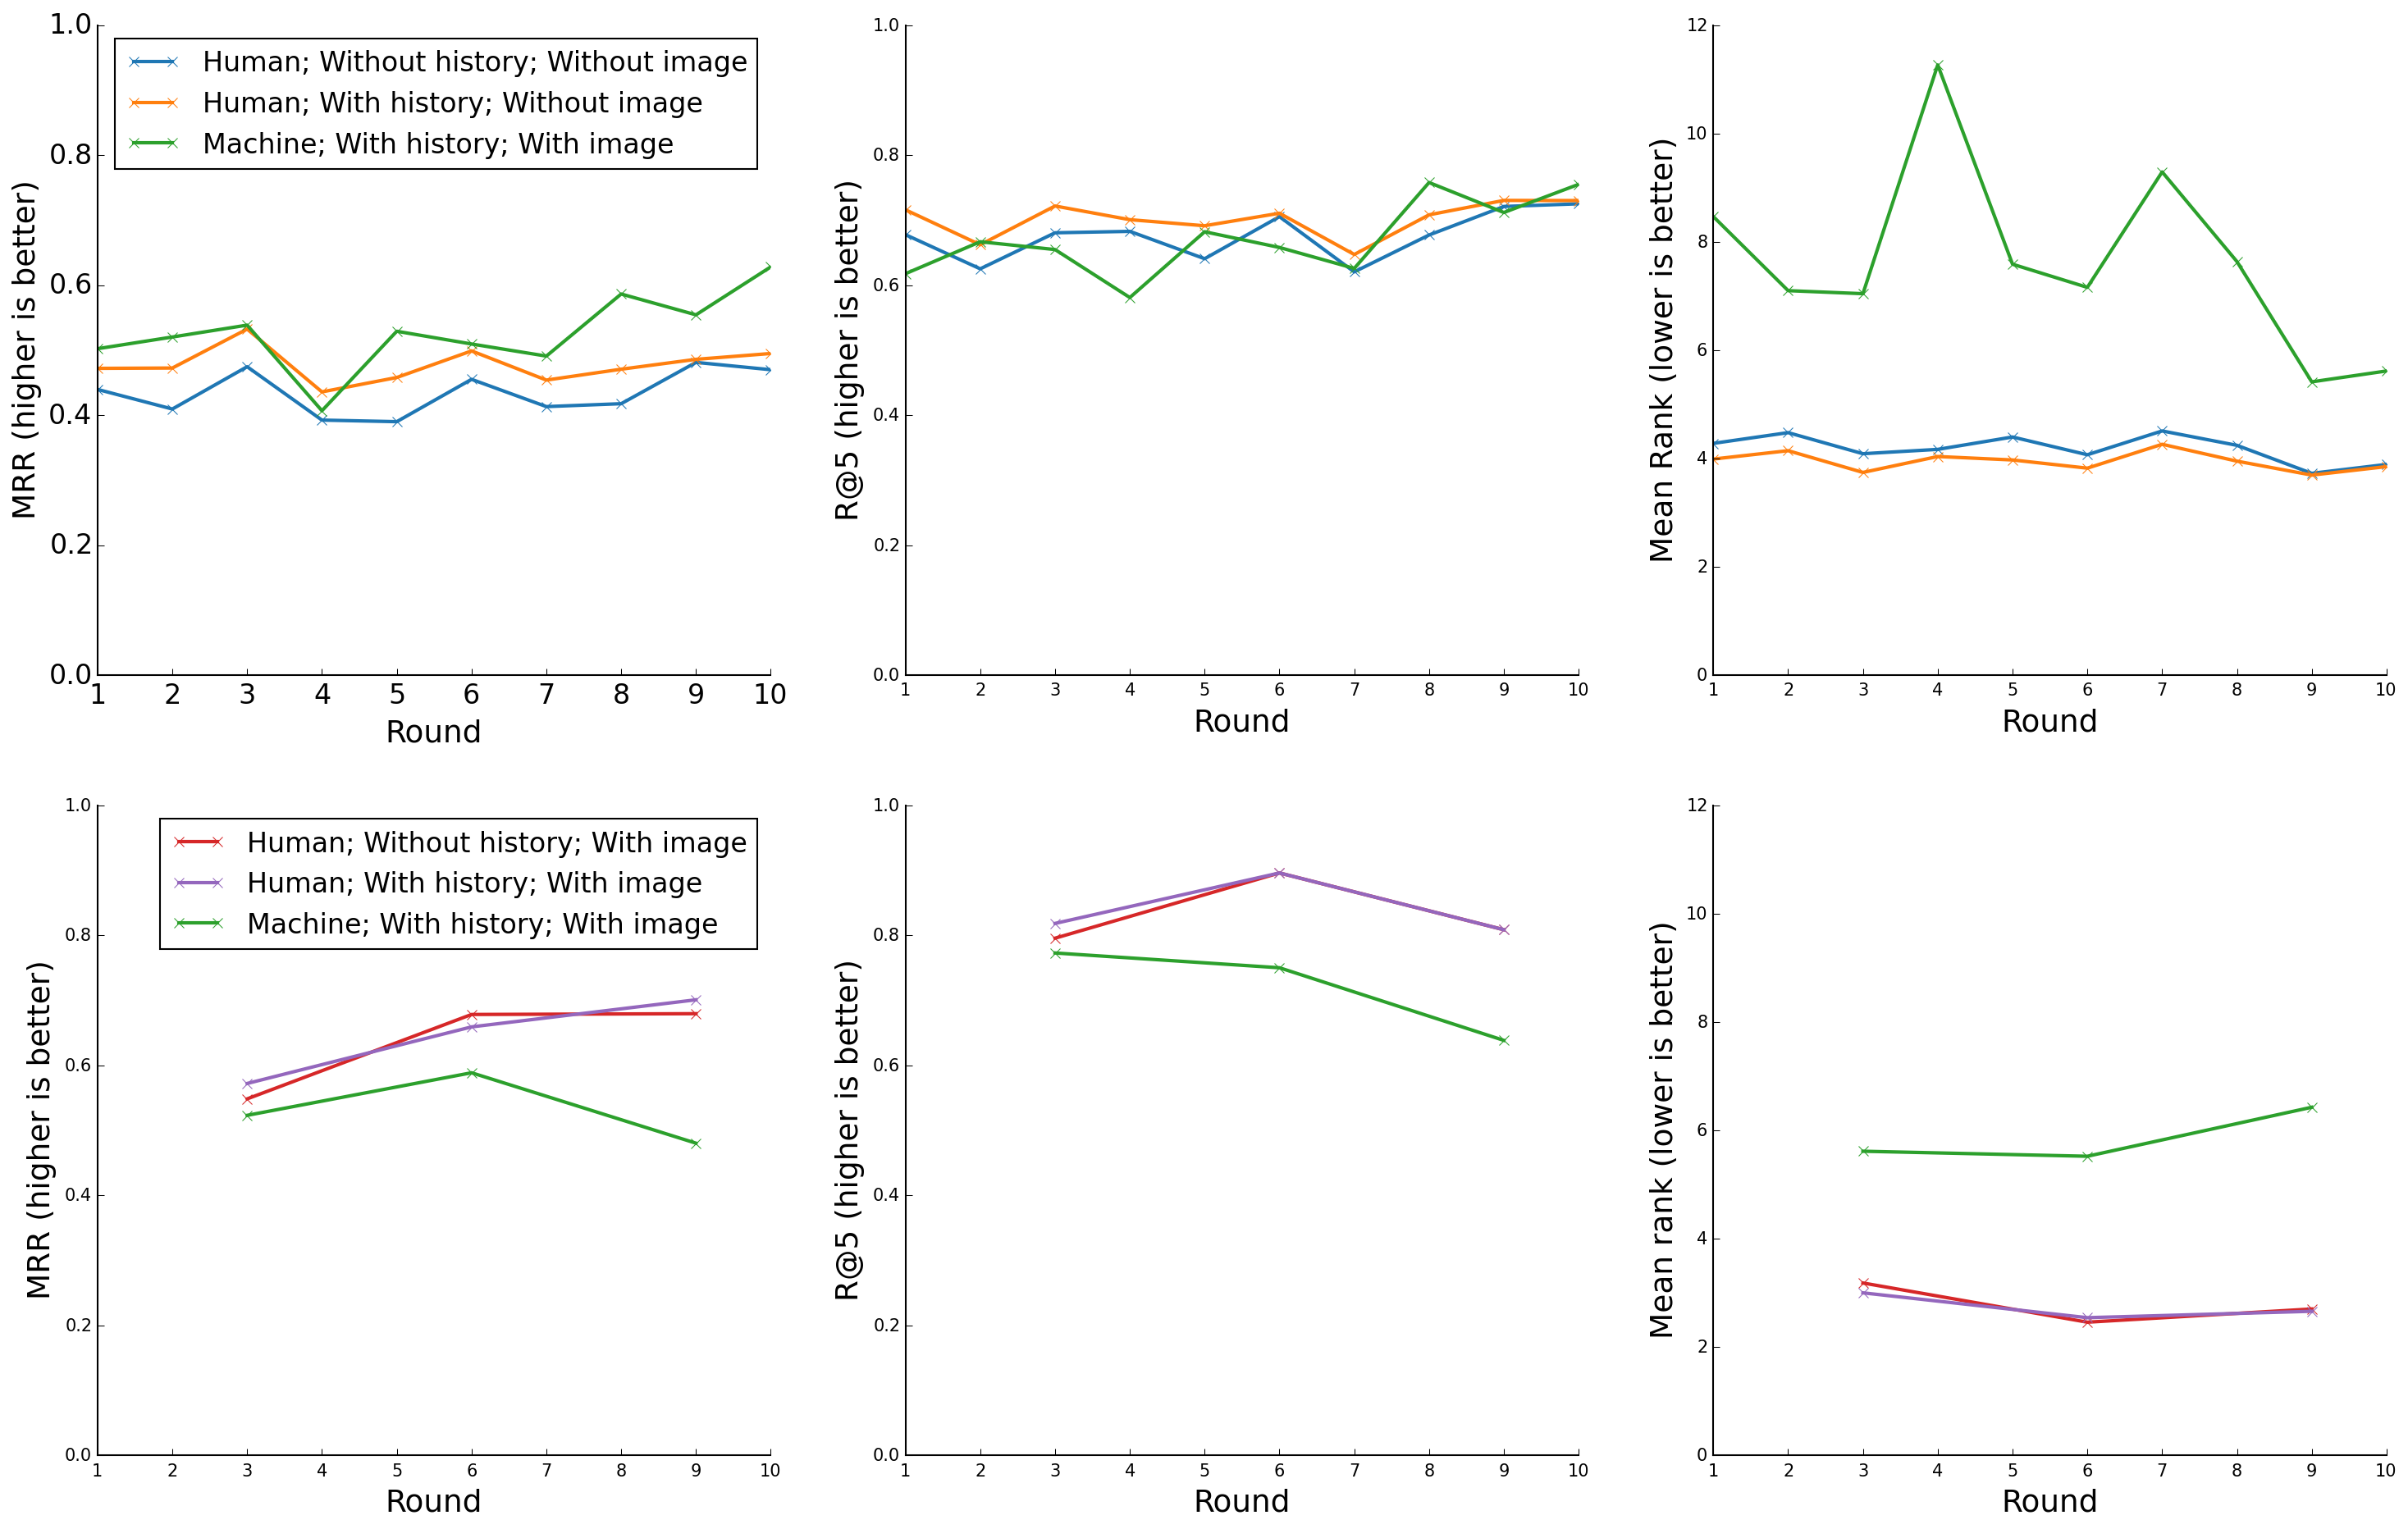}
    \caption{Human accuracy trends on MRR, R@5 and Mean Rank compared to the LF-QIH-Dis model}
    \label{fig:human_acc}
\end{figure}

\begin{figure*}[t]
		\centering
		\includegraphics[width=0.9\textwidth]{figures/final/topa_hist.png}
		\caption{Most frequent answer responses except for `yes'/`no'}
		\label{fig:top_answers}
\end{figure*}

As shown in the appendix, our final interface stated \todo{explain this further, include complete instructions}:
\begin{center}
\fbox{
\parbox{0.45\textwidth}
{``\emph{Your objective is to ask questions about the image\\ that help you imagine the scene better.}''}}
\end{center}

\section{Experimental Details}
\label{sec:exp-details}
\sk{
In this section, we describe details about our data preprocessing, training procedure and hyperparameter selection.}

%%%%%%%%%%%%%%%%%%%%%%%%%%%%%%%%%%%%%%%%%%%%%%%%%%%%%%%%%%
\textbf{Splits.}
%%%%%%%%%%%%%%%%%%%%%%%%%%%%%%%%%%%%%%%%%%%%%%%%%%%%%%%%%%%
\sk{
Recall that \vd v0.5 contained 58k \dialogs on COCO-\train and 10k on COCO-\val images, at the time of submission.
We split the 58k into 50k for training, 8k for validation, and use the 10k as test.
We divide the collected 58k \train set into \train and \val splits of 50k and 8k \dialogs.
To select hyperparameters, we use MRR criterion for early stopping on \val set. }

%%%%%%%%%%%%%%%%%%%%%%%%%%%%%%%%%%%%%%%%%%%%%%%%%%%%%%%%%%
 \textbf{Preprocessing.}
 %%%%%%%%%%%%%%%%%%%%%%%%%%%%%%%%%%%%%%%%%%%%%%%%%%%%%%%%%%%
\sk{
 %We perform the following preprocessing on \vd:
 We spell-correct \vd data using the Bing API~\cite{bing_spellapi}.
 Following VQA, we lowercase all questions and answers,
 convert digits to words, and remove contractions, before tokenizing using the Python NLTK~\cite{nltk}.
 We then construct a dictionary of words that appear at least five times in the train set, giving us a vocabulary of around $7.5$k.}

 %%%%%%%%%%%%%%%%%%%%%%%%%%%%%%%%%%%%%%%%%%%%%%%%%%%%%%%%%%%
 \textbf{Training.}
 %%%%%%%%%%%%%%%%%%%%%%%%%%%%%%%%%%%%%%%%%%%%%%%%%%%%%%%%%%%
\sk{
All our models are implemented in Torch~\cite{torch}. %, an open-source deep learning framework.
 Model hyperparameters are chosen by early stopping on \val based on the Mean Reciprocal Rank (MRR) metric.
 %, leading to different settings for discriminative and generative decoders as shown below.
 %\textbf{Models with generative decoder:} All of question LSTM, history LSTM and decoder LSTM have 2 layers with a hidden size of $512$.
 All LSTMs are 2-layered with $512$-dim hidden states.
 We learn $300$-dim embeddings for words and images.
 These word embeddings are shared across question, history, and decoder LSTMs.
 For models with generative decoders, we use Adam~\cite{kingma_iclr15} with a learning rate of $10^{-3}$.
 %decaying by a factor of approx.~$2/3$ every epoch, upto a minimum rate of $5\times10^{-5}$.
 %that decays by a factor of about $2/3$ every epoch, upto a minimum rate of $5\times10^{-5}$,
 For discriminative decoders, we use SGD+Nesterov momentum with a learning rate of $0.1$.
 Gradients at each iterations are clamped to $[-5, 5]$ to avoid explosion.
 Our code, architectures, and trained models will be publicly available.}

 \begin{figure*}[]
    \centering
    \includegraphics[width=\linewidth]{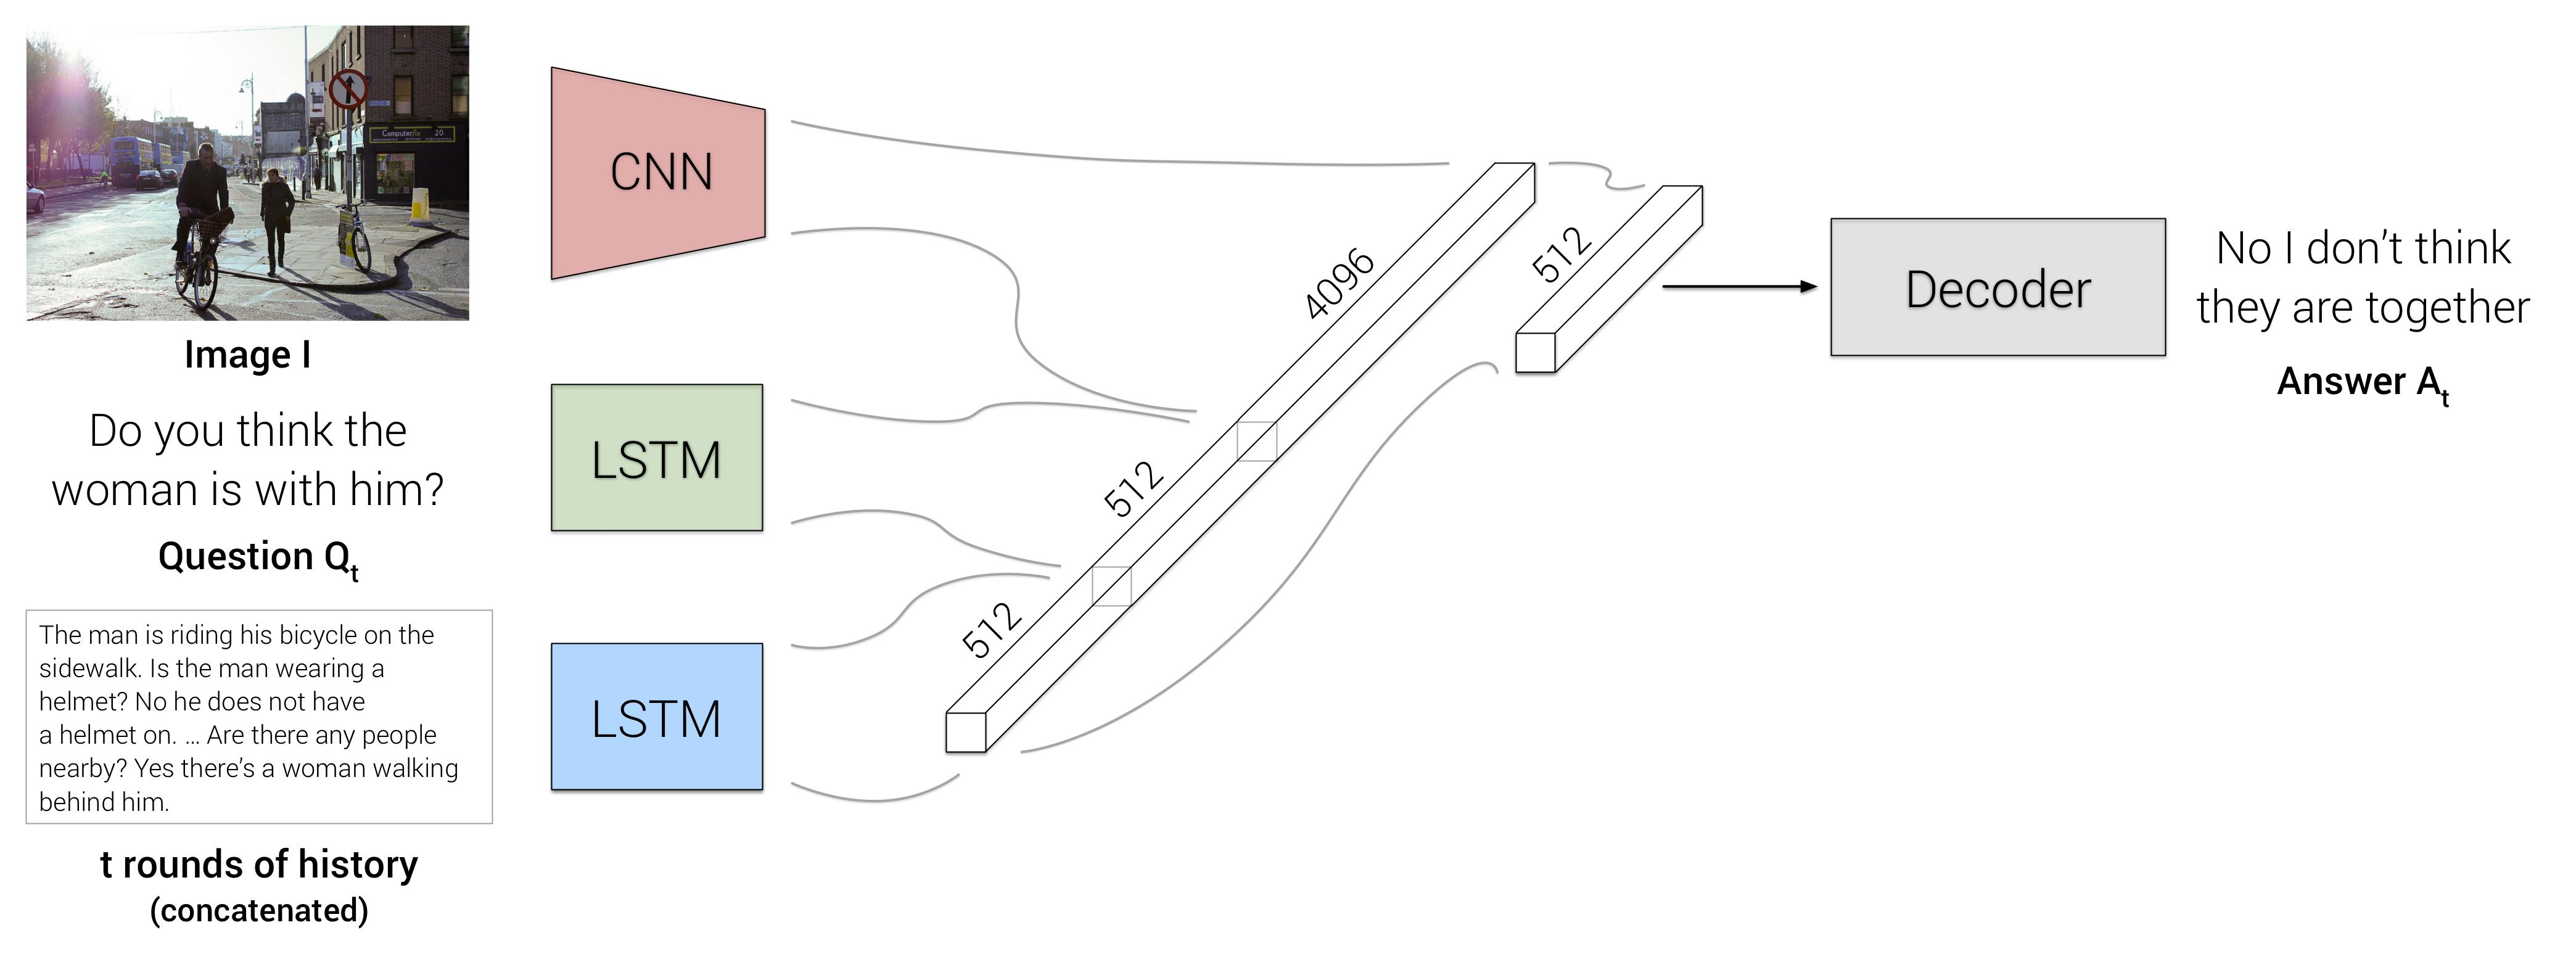}
    \caption{Late Fusion encoder}
    \label{fig:lf_enc}
\end{figure*}

\begin{figure*}[t]
    \centering
    \includegraphics[width=\linewidth]{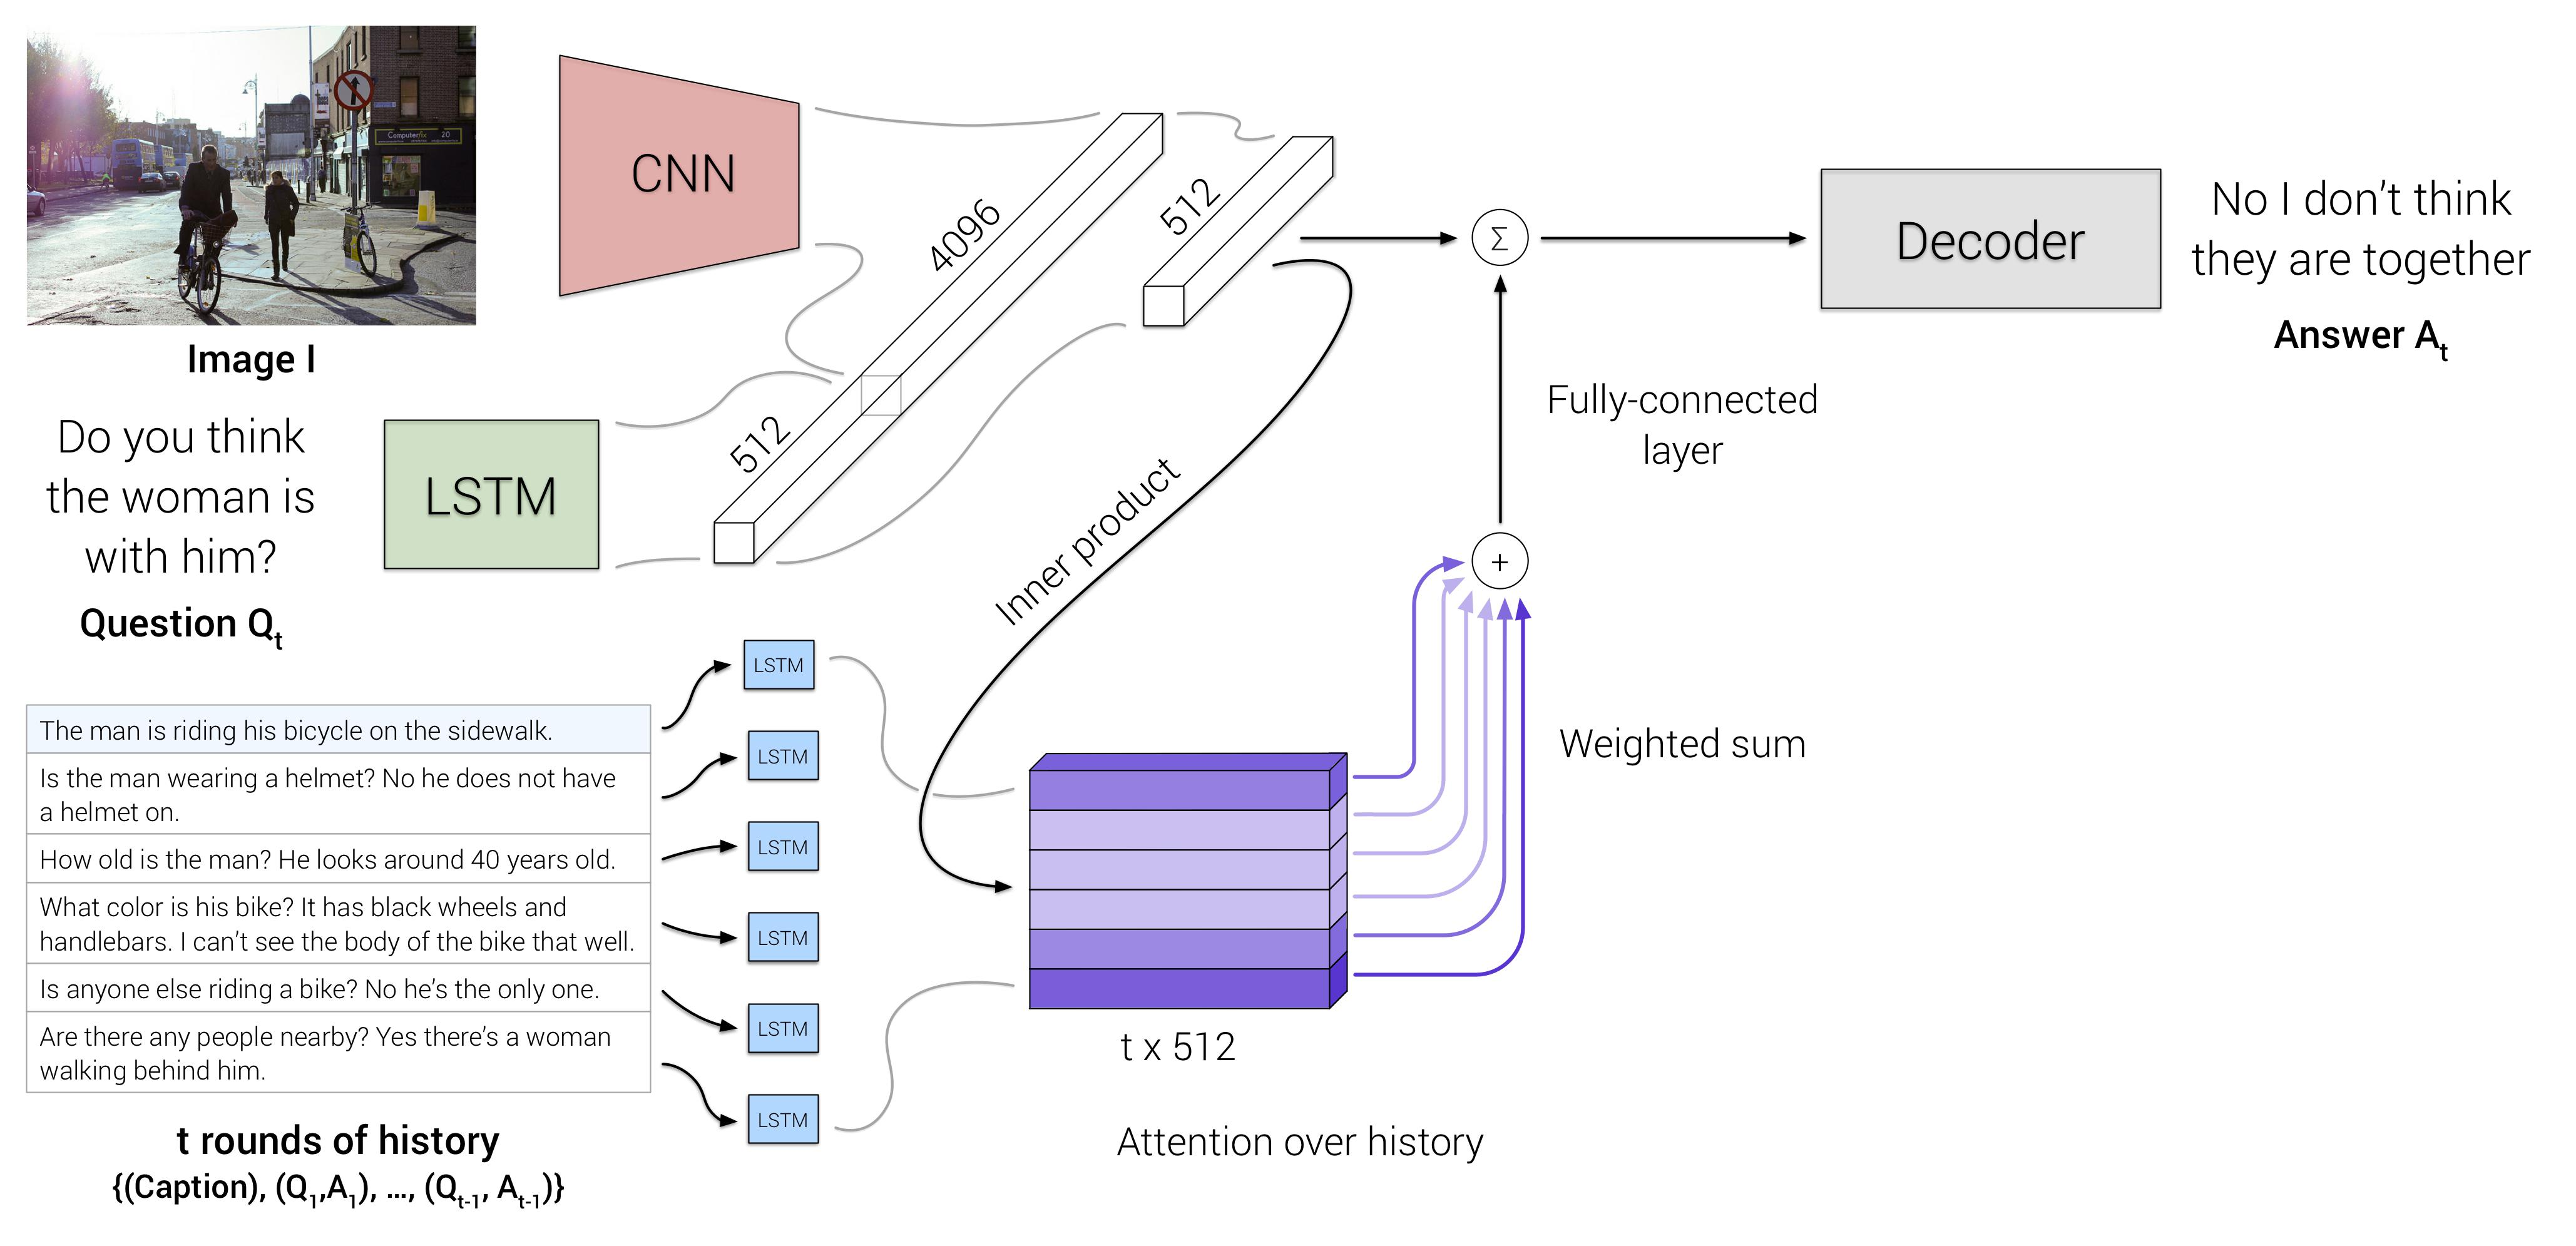}
    \caption{Memory Network encoder}
    \label{fig:mn_enc}
\end{figure*}
